# Supplementary material for: Oxygen vacancy formation and electronic reconstruction in strained LaNiO$_3$ and LaNiO$_3$/LaAlO$_3$ superlattices
Source: arXiv:2206.11028 ancillary file (2022-06-22)
Supplement: Supplementary file 1 [file Supplement.pdf]

# Oxygen vacancy formation and electronic reconstruction in strained $LaNiO_3$ and $LaNiO_3/LaAlO_3$ superlattices
# – Supplemental Material –

Benjamin Geisler, Simon Follmann, and Rossitza Pentcheva
*Department of Physics and Center for Nanointegration (CENIDE), Universität Duisburg-Essen, Lotharstr. 1, 47057 Duisburg, Germany*

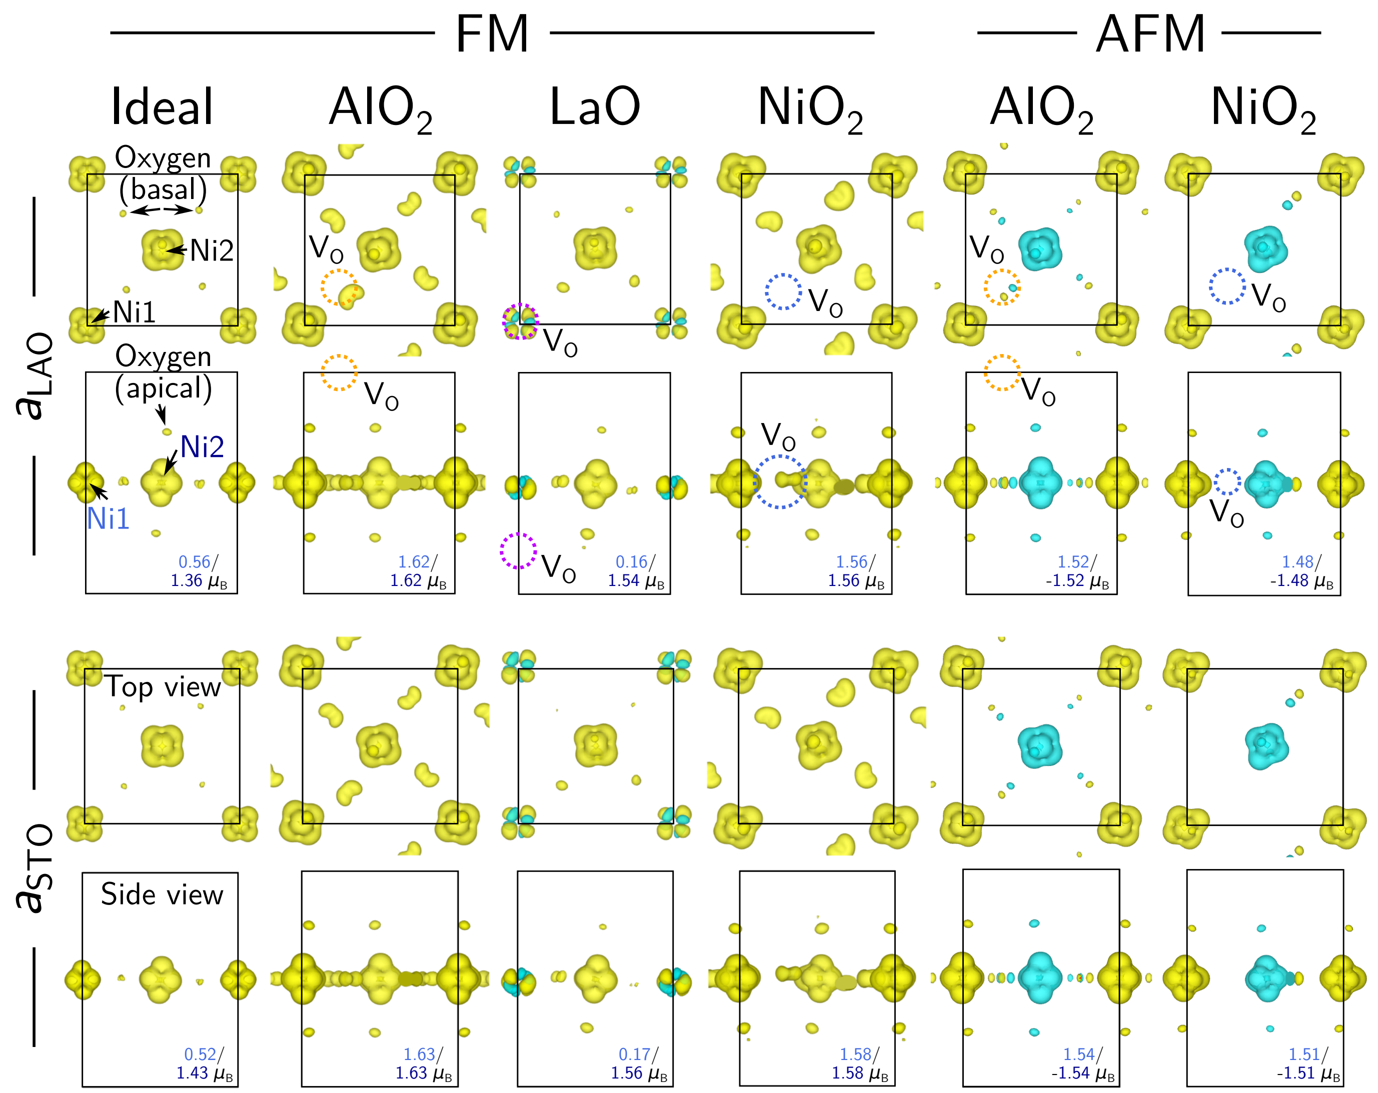


Figure 1. Spin densities (top and side views) of $(LNO)_1/(LAO)_1(001)$ SLs for 8.3% $V_O$ concentration at compressive ($a_{LAO}$, top rows) and tensile ($a_{STO}$, bottom rows) epitaxial strain, comparing the impact of $V_O$ in different layers to the ideal case (yellow: positive contributions; blue: negative contributions). We use the same density value for the isosurfaces (0.02 a.u.$^{-3}$) in all cases. See also Figs. 2 and 3.

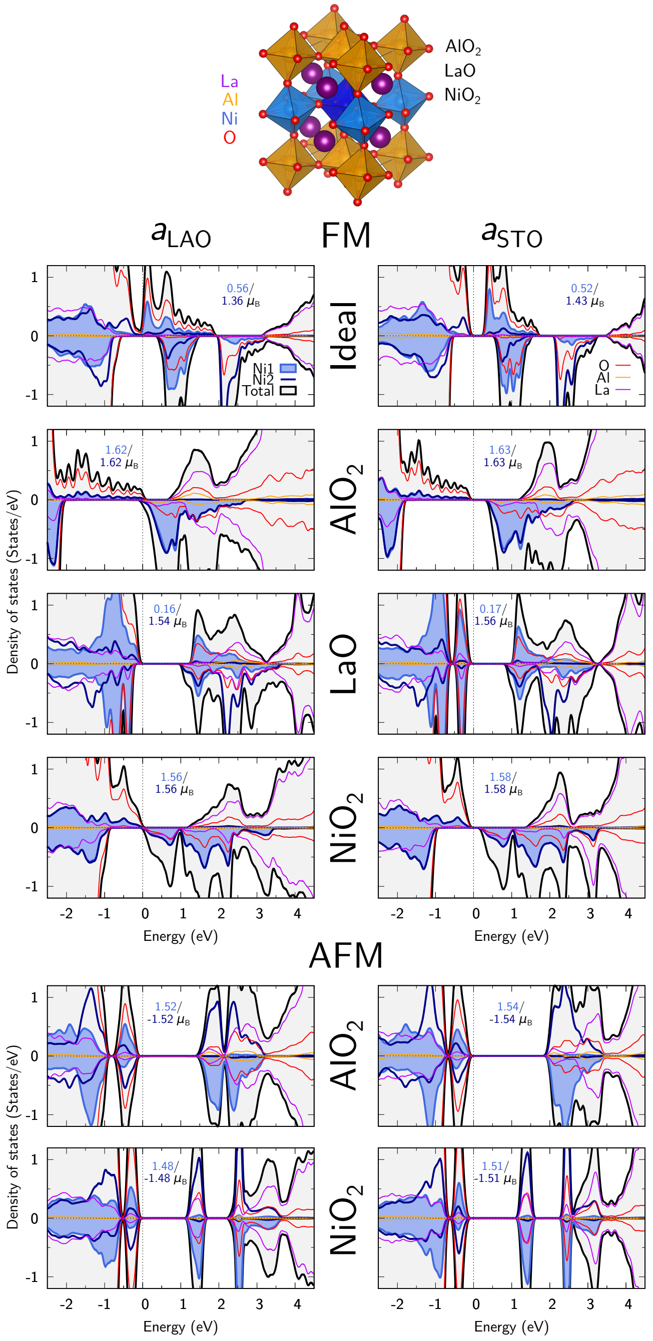


Figure 2. Spin- and element-resolved densities of states of $(LNO)_1/(LAO)_1(001)$ SLs for 8.3% $V_O$ concentration at compressive ($a_{LAO}$, left) and tensile ($a_{STO}$, right) epitaxial strain, comparing the impact of $V_O$ in different layers to the ideal case. The Ni1, Ni2, O, La, and Al curves have been obtained by averaging over all respective sites and are normalized per formula unit. We find AFM to be the ground state for $V_O$ in the $AlO_2$ and $NiO_2$ layers. See also Fig. 3.

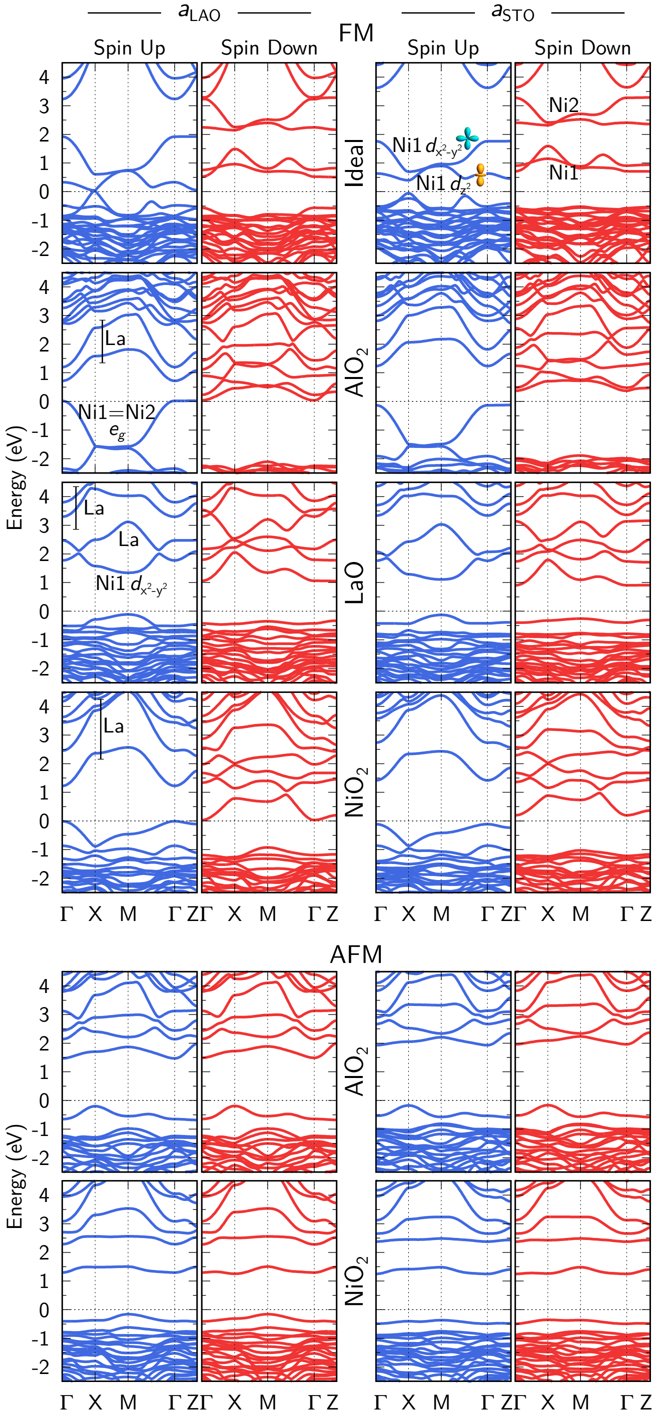


Figure 3. Spin-resolved band structures of $(LNO)_1/(LAO)_1(001)$ SLs for 8.3% $V_O$ concentration at compressive ($a_{LAO}$, left) and tensile ($a_{STO}$, right) epitaxial strain, comparing the impact of $V_O$ in different layers to the ideal case. See also Fig. 2.

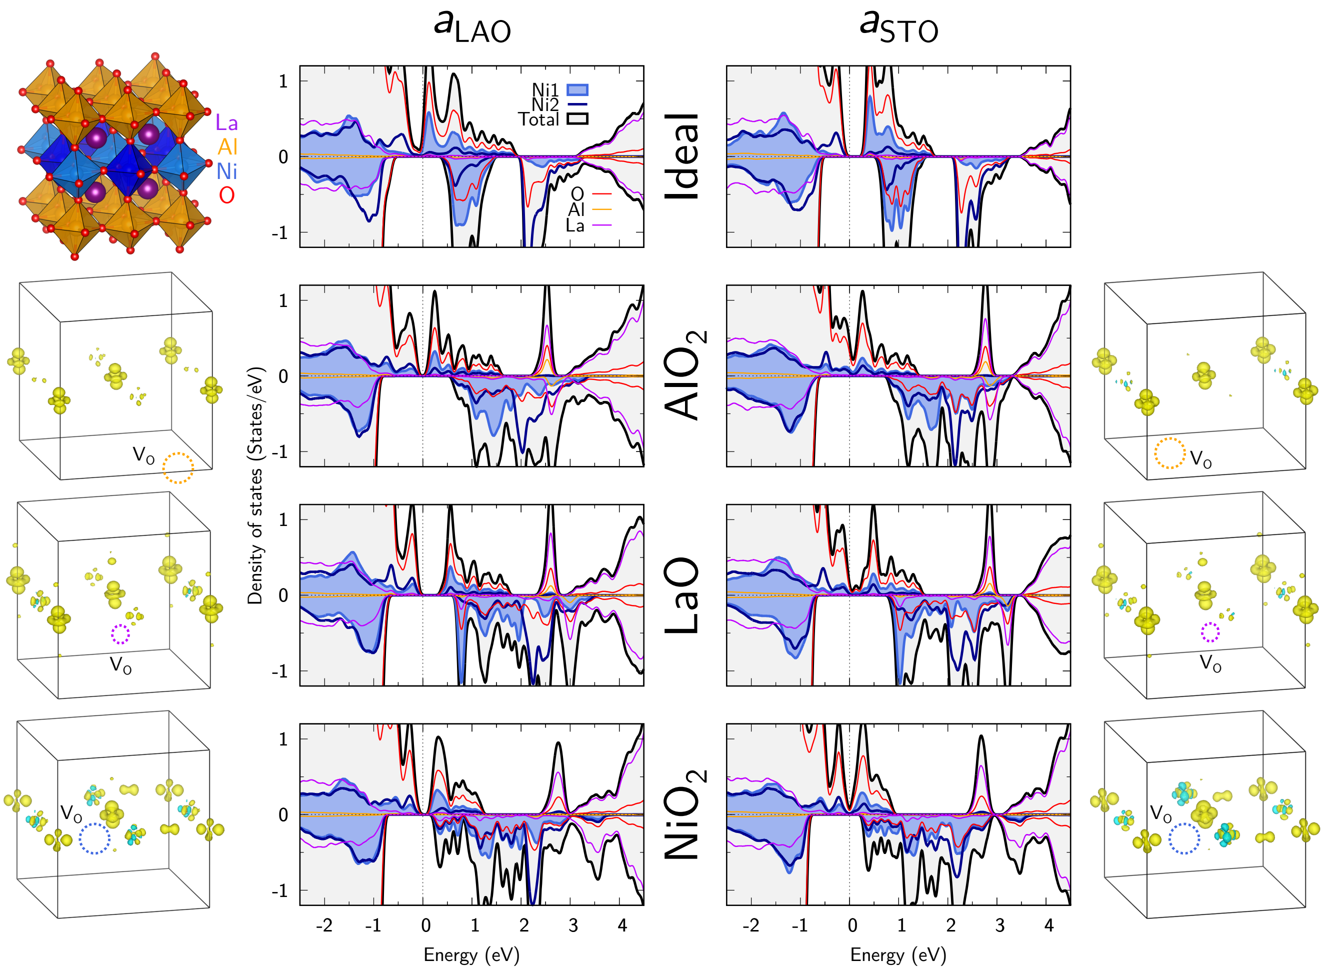


Figure 4. Spin- and element-resolved densities of states of $(LNO)_1/(LAO)_1(001)$ SLs for 4.2% $V_O$ concentration at compressive ($a_{LAO}$, left) and tensile ($a_{STO}$, right) epitaxial strain, comparing the impact of $V_O$ in different layers to the ideal case. The outer panels show spin density *differences* with respect to the ideal case, i.e., the vacancy-induced local changes in orbital occupation (yellow: increase; blue: decrease).

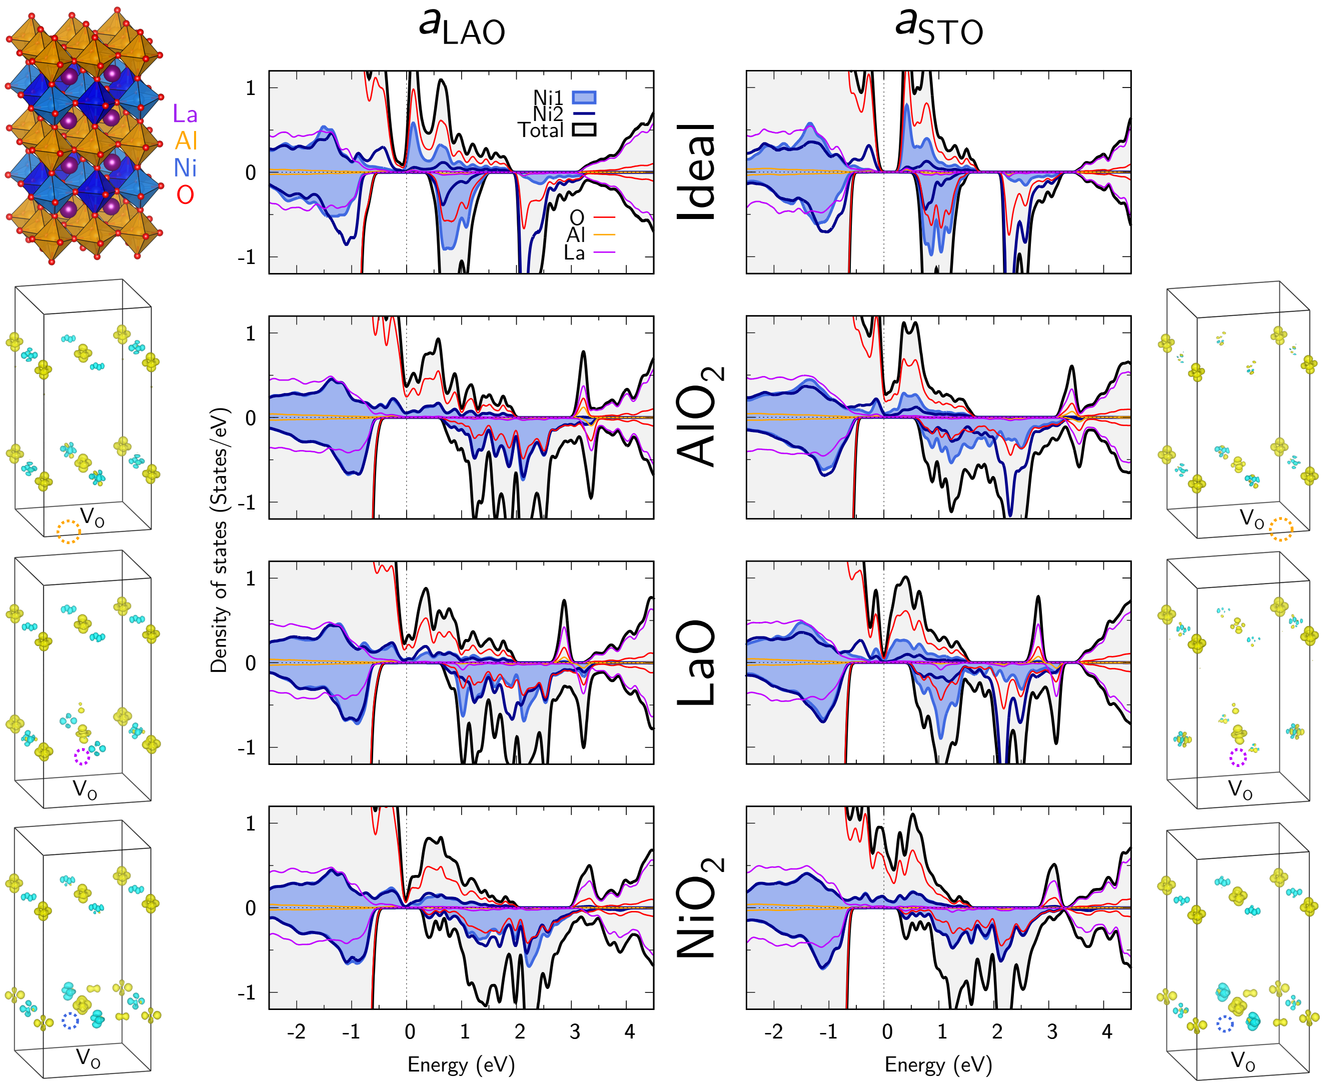


Figure 5. Spin- and element-resolved densities of states of $(\mathrm{LNO})_1/(\mathrm{LAO})_1(001)$ SLs for 2.1% $\mathrm{V_O}$ concentration at compressive ($a_{\mathrm{LAO}}$, left) and tensile ($a_{\mathrm{STO}}$, right) epitaxial strain, comparing the impact of $\mathrm{V_O}$ in different layers to the ideal case. The outer panels show spin density *differences* with respect to the ideal case, i.e., the vacancy-induced local changes in orbital occupation (yellow: increase; blue: decrease).

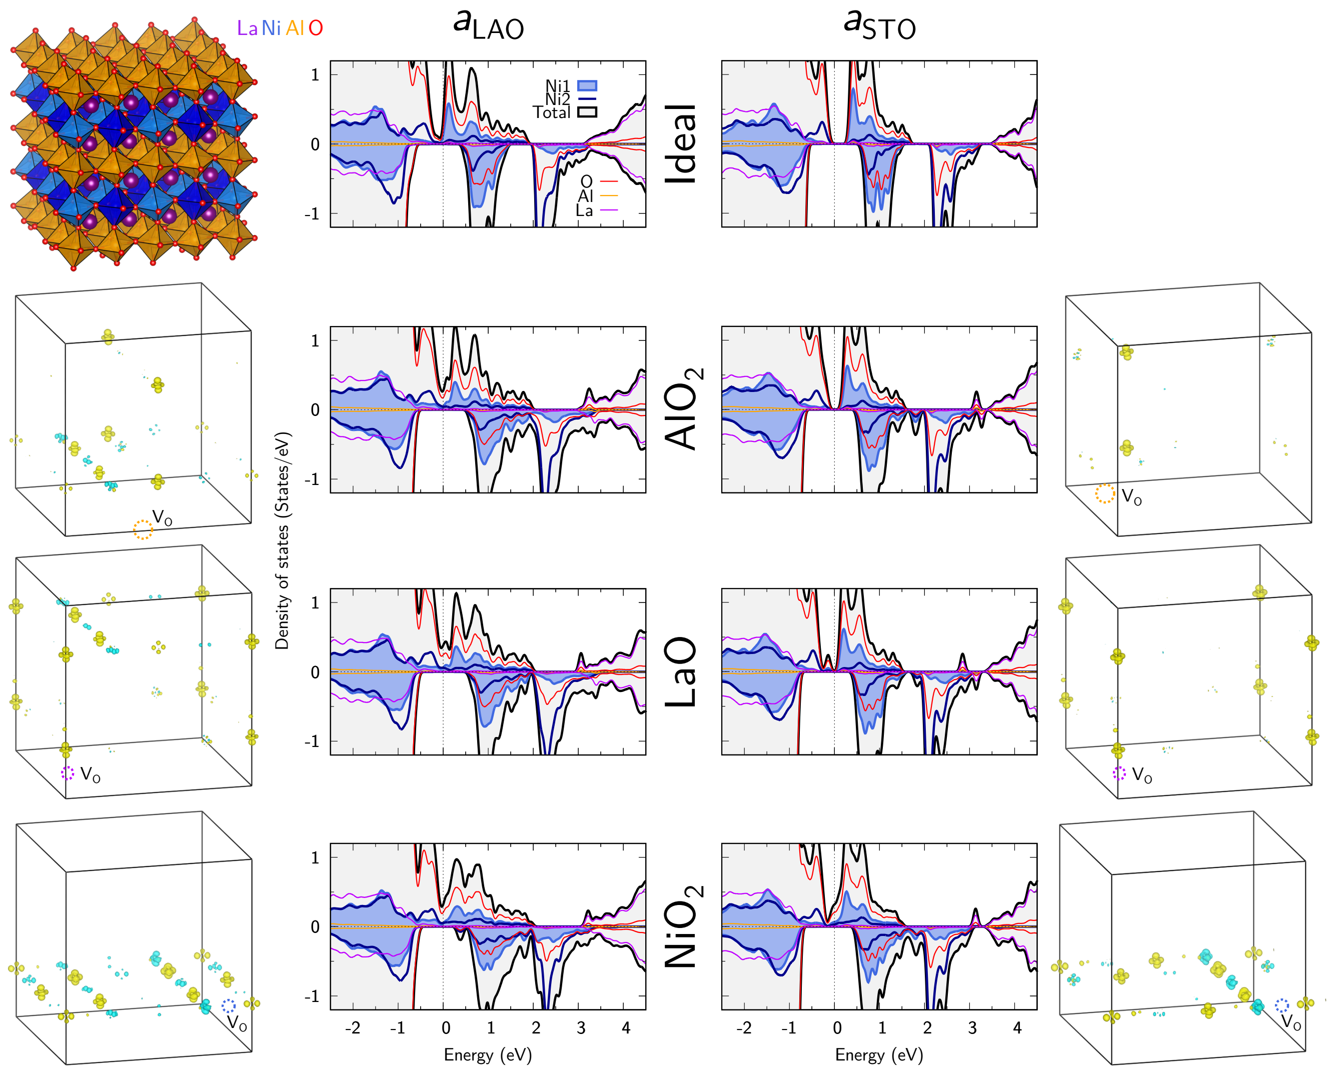


Figure 6. Spin- and element-resolved densities of states of $(\mathrm{LNO})_1/(\mathrm{LAO})_1(001)$ SLs for $0.5\%$ $\mathrm{V_O}$ concentration at compressive ($a_{\mathrm{LAO}}$, left) and tensile ($a_{\mathrm{STO}}$, right) epitaxial strain, comparing the impact of $\mathrm{V_O}$ in different layers to the ideal case. The outer panels show spin density *differences* with respect to the ideal case, i.e., the vacancy-induced local changes in orbital occupation (yellow: increase; blue: decrease).
